# Supplementary material for: CONNA: Addressing Name Disambiguation on The Fly
Source: arXiv:1910.12202 source file (2020-09-14)
Supplement: Supplementary file 1 [file appendix.tex]

\begin{appendices}
\section{}
\subsection{Implementation Details}

\vpara{Matching Component.}
For the multi-field  modeling, we divide the attributes of a paper into two fields: the author names and the words in all the other attributes, including the paper's title and keywords, the published venue, and the target author's affiliation. We separate author names from others as author names have no literal or semantic overlaps with them, while other attributes are merged due to the overlaps of similar words. 

The special symbols such as ``-" and ``."  in author names and words are removed.  The stop words are removed and the stems of the words are extracted. 
We pre-train an embedding for each author name and word. Specifically, we use Word2Vec to train a name embedding in the context of all the coauthors' names in a paper, and train a word embedding in the context of all the other occurred words in title, keywords, venue and affiliation.
We set the dimension of the embedding as 100. To enable matrix operation, for each paper or candidate person, we limit the maximal number of author names to 100, the maximal number of words to 500, and the maximal number of papers published by each person to 100. 

The hyper-parameters of the RBF kernel functions are set the same as~\cite{xiong2017end}. We use 11 RBF kernel functions, with the hyper-parameters $\mu=\{1, 0.9, 0.7, 0.5, 0.3, 0.1, -0.1, -0.3, -0.5, -0.7, -0.9\}$  and $\sigma = \{10^{-3}, 0.1, 0.1, 0.1, 0.1, 0.1, 0.1, 0.1, 0.1, 0.1, 0.1\}$, where the kernel with $\mu=1.0$ and $\sigma=10^{-3}$ captures the exact matches, and other kernels capture soft matches between tokens.

\hide{
The details of the matching component include:

\begin{enumerate}
	\item We first lookup the embeddings for each author name and word from a pre-trained embedding corpus;
	\item Based on the pre-trained embeddings, for each field of the attributes, we generate a similarity embedding between the target paper  and each paper of the candidate person by the basic profile model;
	\item For a pair of the target paper and a paper of the candidate, we concatenate the similarity embeddings of different fields by the proposed attention mechanism in the multi-field profile model;
	\item For a pair of the target paper and the candidate, we concatenate similarity embeddings of different papers of the candidate by the proposed attention mechanism in the multi-field multi-instance model;
	\item We concatenate the multi-field profile feature vector with multi-field multi-instance feature vector to create the final similarity embedding;
%	\item we concatenate the multi-field multi-instance feature vector with the 17 manually extracted features in Table~\ref{tb:features} to create the final similarity embedding;
	\item A non-linear function $g$ is to used to transform the similarity embedding to a one-dimension matching score;
	\item The triplet loss in Eq. (6) is used to train the matching component.
\end{enumerate}
}
The model parameters $\Theta$ include the word/author embeddings which are fine-tuned in our model, the parameters of the attention mechanism and the parameters of the non-linear function $g$ that is used to transform the similarity embedding into a matching score. For training, the mini-batch is set as 80. The learning rate is set as 0.001.

\vpara{Decision Component.}
The decision component is a basic multiple layer perceptron, with four-layer full connections followed by a ReLU function. Other complex models obtain the similar performance with the basic MLP. 
The model parameters $\Phi$ include the the parameters of the basic MLP.
For training, the size of the mini-batch is set as 128. The learning rate is set as 0.001.

%\vpara{The Joint Model.} After the matching and the decision components are pre-trained, we give a reward 0 to the wrongly-predicted instances and a reward 1 to the rightly-predicted instances in the training data to guide the updating of the matching component. The decision component is continuously updated on the new training data with the top-matched wrong persons and the similarity embeddings updated by the matching component. The process is repeated until the two components converge. The learning rate is set as 0.0001 for both the matching and the decision component in the joint fine-tuning process.

\subsection{Running Environment}
We implement the model by Tensorflow and run the code on an Enterprise Linux Server with 40 Intel(R) Xeon(R) CPU cores (E5-2640 v4 @ 2.40GHz  and 252G memory) and 1 NVIDIA Tesla V100 GPU core (32G memory).

\subsection{Baselines}
\label{sec:baseline}
%We use the SVM implementation in the Python scikit-learn package. 
The features extracted for SVM is shown in Table~\ref{tb:features}. 
%The codes of Camel\footnote{https://github.com/chuxuzhang/code\_Camel\_WWW2018}, HetNetE\footnote{https://github.com/chentingpc/GuidedHeteEmbedding} and GML\footnote{https://github.com/neozhangthe1/disambiguation/} are provided by the authors of the original papers. 

{\small \begin{table}[t]
		{\caption{Features extracted for the SVM model. \small{$p$: target paper, $a$: target author in $p$, $c$: candidate person.} }\label{tb:features}} 
		\vspace{-0.08in}
		{%
			{
				\setlength{\extrarowheight}{1pt}
				\begin{tabular}{
						@{}c@{ } l@{}}
					\noalign{ \hrule height 1pt}
					\textbf{No.}   & \textbf{Feature description} \\ \hline
					\textbf{1}      &  Paper number of $c$\\ 
					\textbf{2}      &  Distinct venue number of $c$\\ \hdashline
					\textbf{3}      &  Frequency of $a$'s coauthors in $c$\\  
					\textbf{4}      &  Ratio of $a$'s coauthors in $p$'s author names\\ 
					\textbf{5}      &  Ratio of $a$'s coauthors  in $c$'s author names\\ \hdashline		
					\textbf{6}      &  Frequency of $a$'s affiliation in $c$\\ 
					\textbf{7}      &  Ratio of $a$'s affiliation in the same name's affiliations in $c$\\ 
					\textbf{8}      &  Cosine similarity of the affiliations between $a$ and $c$'s same names\\ 
					\textbf{9}      &  Jaccards similarity of the affiliations between $a$ and $c$'s same names\\  \hdashline
					\textbf{10}      &  Frequency of $p$'s venue in $c$\\ 
					\textbf{11}      &  Ratio of $p$'s venue in $c$\\ 
					\textbf{12}      &  Cosine similarity between $p$'s venue and $c$'s venues \\ 
					\textbf{13}      &  Jaccards similarity between $p$'s venue and $c$'s venues \\  \hdashline
					\textbf{14}      &  Cosine similarity between $p$'s title and $c$'s titles\\ 
					\textbf{15}      &  Jaccards similarity between $p$'s title and $c$'s titles\\  
					\textbf{16}      &  Cosine similarity between $p$'s keywords and $c$'s keywords\\ 
					\textbf{17}      &  Jaccards similarity between $p$'s keywords and $c$'s keywords\\  
					
					\noalign{\hrule height 1pt}
				\end{tabular}}
				
			}
		\end{table} }

\end{appendices}
